# Supplementary material for: The Spherical Grasshopper Problem
Source: arXiv:2307.05359 source file (2023-07-08)
Supplement: Supplementary file 1 [file 21Appendix.tex]

\appendix
\chapter{Extra Information}
Some more text ...
